# Supplementary material for: Interactive Training: Feedback-Driven Neural Network Optimization
Source: arXiv:2510.02297 source file (2025-10-02)
Supplement: Supplementary file 1 [file data_creation_process.tex]

\definecolor{borderblue}{RGB}{34,51,103}    % dark frame
\definecolor{bggray}{RGB}{245,247,250}

\section{Data Construction Process}
\label{appendix:data_creation}
In this part, we explain in detail how we create the dataset. We start with WildChat-Full dataset which contains around 990K conversations. 

\subsection{Pre-processing and De-duplication}
We begin by de-duplicating the full WildChat dataset using MinHash and Locality-Sensitive Hashing (LSH), following the approach described in \citet{huggingface_dedup_2023}. For MinHash, we use 4-grams ($k = 4$) and 9 permutations ($p = 9$). For LSH, we set the band size to $b = 7$ and the row size to $r = 3$. After de-duplication, approximately 520K conversations remain.

Next, we tokenize all conversations using the LLaMA 3 tokenizer \cite{grattafiori2024llama3herdmodels} and discard those exceeding 4,096 tokens. Users are identified based on a combination of hashed IP addresses and HTTP request headers, and each user is assigned a randomized username. Users with fewer than 10 sessions are considered inactive, and all their conversations are removed.

After filtering by conversation length and user activity, around 220K conversations remain. All subsequent processing steps are performed on this filtered dataset.

\begin{figure*}[htbp]
    \centering
   \begin{tcolorbox}[colframe=borderblue, colback=bggray, left=1mm, right=1mm, top=0.5mm, bottom=0.5mm]
    \inputminted[fontsize=\scriptsize, breaklines, breakanywhere, breaksymbolleft={}]{markdown}{appendix/prompts/extract_keywords_and_summary.md}
\end{tcolorbox}
    \caption{Prompt for keywords extraction and summarization. }
    \label{fig:prompt_extraction}
\end{figure*}

\begin{algorithm*}[htbp]
\caption{TnT-LLM: Taxonomy Generation Phase}
\label{alg:tnt-llm-taxonomy-topic}
\begin{algorithmic}[1]
\Statex \textbf{Input:} Max round of iteration $N$, Batch size $B$, Conversations summaries $C$, Summary embeddings $E$, 2Number of cluster of KMeans $K$, Initial taxonomy generation prompt $P_{\text{initial, topic}}$, Taxonomy update prompt $P_{\text{update, topic}}$
\Statex \textbf{Output:} Label taxonomy $T$

\State Partition summaries $C$ into $K$ clusters $\{D_1, \dots, D_K\}$ using KMeans on $E$.
\State Initialize taxonomy $T \leftarrow \emptyset$.
\State Initialize cursors for round-robin sampling from each cluster $D_k$.

\For{$n \leftarrow 1 \text{ to } N$}
    \State $S_{batch} \leftarrow \emptyset$
    \State Select up to $B$ summaries for $S_{batch}$ by sampling from clusters $\{D_k\}$ in a round-robin fashion without replacement, advancing cursors.
    
    \If{$S_{batch}$ is empty} \Comment{No more summaries available for sampling}
        \State \textbf{break}
    \EndIf

    \If{$n = 1$}
        \State $T \leftarrow \text{CallLLM}(P_{\text{initial, topic}}, S_{batch})$
    \Else
        \State $T, \text{score} \leftarrow \text{CallLLM}(P_{\text{update, topic}}, S_{batch}, T)$ \Comment{Update existing $T$}
    \EndIf

    \If{score not improve for 3 iteration}
        \State \textbf{break}
    \EndIf
\EndFor
\State \Return $T$

\end{algorithmic}
\end{algorithm*}

\subsection{LLM-based keywords and summarization extraction}

To perform TnT-LLM for topic discovery, we begin by extracting keywords and summaries from raw conversations. Specifically, we prompt GPT-4o to generate both the keyword set and a concise summarization of each conversation. The extracted keywords span a diverse set of semantic types, including persons, technologies, scientific terms, foods, demographic terms, organizations, locations, events, artworks, programming languages, product brands, and financial terms. The complete prompt used for this extraction process is shown in \Cref{fig:prompt_extraction}.

\begin{figure*}[htbp]
    \centering
   \begin{tcolorbox}[colframe=borderblue, colback=bggray, left=1mm, right=1mm, top=0.5mm, bottom=0.5mm]
\inputminted[fontsize=\scriptsize, breaklines, breakanywhere, breaksymbolleft={}]{markdown}{appendix/prompts/topic_initial_taxonomy_generation.md}
\end{tcolorbox}
    \caption{Initial Taxonomy Generation Prompt}
    \label{fig:topic_initial}
\end{figure*}

\begin{figure*}[htbp]
    \centering
   \begin{tcolorbox}[colframe=borderblue, colback=bggray, left=1mm, right=1mm, top=0.5mm, bottom=0.5mm]
\inputminted[fontsize=\scriptsize, breaklines, breakanywhere, breaksymbolleft={}]{markdown}{appendix/prompts/topic_taxonomy_update_part1.md}
\end{tcolorbox}
\end{figure*}

\begin{figure*}[htbp]
    \centering
   \begin{tcolorbox}[colframe=borderblue, colback=bggray, left=1mm, right=1mm, top=0.5mm, bottom=0.5mm]
\inputminted[fontsize=\scriptsize, breaklines, breakanywhere, breaksymbolleft={}]{markdown}{appendix/prompts/topic_taxonomy_update_part2.md}
\end{tcolorbox}
    \caption{Taxonomy Update Prompt}
    \label{fig:topic_update}
\end{figure*}

\subsection{TnT-LLM based Topic and Subtopic Discovery and Assignment}
\subsubsection{Topic Discovery and Assignment}
\paragraph{Topic Taxonomy Generation}
We largely follow the pipeline of TnT-LLM \cite{wan2024tntllmtextminingscale} to identify topics within the dataset. Rather than randomly sampling from a large corpus, we first obtain the textual embeddings of conversation summaries using the \texttt{BAAI/bge-en-icl} model \cite{li2024makingtextembeddersfewshot}. We then perform clustering on these embeddings to guide our sampling, ensuring a diverse selection across different semantic regions. This step is added to enhance topic diversity in the sampled subset.

Subsequently, we apply the topic discovery algorithm detailed in \Cref{alg:tnt-llm-taxonomy-topic}. The initial taxonomy generated is visualized in \Cref{fig:topic_initial}, while the prompt used for topic refinement is shown in \Cref{fig:topic_update}. For all topic discovery steps, we employ GPT-4o as the underlying language model, using hyperparameters $B=K=500$ and $N=10$. To perform efficient KMeans clustering, we utilize the FAISS library \cite{douze2025faisslibrary}. Unlike the original TnT-LLM method, which relies on LLMs for taxonomy refinement, we manually resolve conflicts and enforce mutual exclusivity among the discovered topics.

\begin{figure*}[htbp]
    \centering
   \begin{tcolorbox}[colframe=borderblue, colback=bggray, left=1mm, right=1mm, top=0.5mm, bottom=0.5mm]
\inputminted[fontsize=\scriptsize, breaklines, breakanywhere, breaksymbolleft={}]{markdown}{appendix/prompts/topic_assignment.md}
\end{tcolorbox}
    \caption{Topic Assignment Prompt}
    \label{fig:topic_assignment}
\end{figure*}

\paragraph{Topic Label Assignment}  Using the generated topics and corresponding taxonomy, we assign a topic ID to each conversation. This assignment process can be formulated as a multi-label classification task. The labeling is performed by GPT-4o using the assignment prompt illustrated in \Cref{fig:topic_assignment}. The prompt is carefully designed to mitigate common errors identified through a manual inspection of a small validation set consisting of 400 examples.

% \begin{algorithm*}[htbp]
% \caption{Subtpic Taxonomy Generation}
% \label{alg:subtopic_taxonomy}
% \begin{algorithmic}[1]
% \Statex \textbf{Input:} Max round of iteration $N$, Batch size $B$, Conversations summaries $C$, Summary embeddings $E$, Number of cluster of KMeans $K$, Initial taxonomy generation prompt $P_{\text{initial, topic}}$, Taxonomy update prompt $P_{\text{update, topic}}$
% \Statex \textbf{Output:} Label taxonomy $T$
% \end{algorithmic}
% \end{algorithm*}

\subsubsection{Subtopic Discovery and  Assignment}
\begin{figure*}[htbp]
    \centering
   \begin{tcolorbox}[colframe=borderblue, colback=bggray, left=1mm, right=1mm, top=0.5mm, bottom=0.5mm]
\inputminted[fontsize=\scriptsize, breaklines, breakanywhere, breaksymbolleft={}]{markdown}{appendix/prompts/aspected_summarize.md}
\end{tcolorbox}
    \caption{Topic Validation and Aspected Summarize Prompt}
    \label{fig:subtopic_aspected_summarize}
\end{figure*}
\paragraph{Subtopic Taxonomy Generation} For each discovered topic, we further identify its subtopics by running TnT-LLM on all conversations classified under that topic. However, subtopic discovery proves to be more challenging. To address this, we adopt a more sophisticated pipeline and employ a stronger model. The following pipeline is specifically designed to facilitate subtopic discovery within each major topic.

\begin{itemize}
    \item[1.] Prompt GPT-4o to check the result of topic assignment and summarize the raw conversation from the perspective of major topic using the prompt shown in \Cref{fig:subtopic_aspected_summarize}. 
    \item[2.] Get the embedding of the summaries that pass checking using \texttt{text-embedding-3-large}.
    \item[3.] Run KMeans use faiss with $K$ in $\{10, 15, 20, 25, 30, 35, 40\}$, find the top 3 best number of centroid $k_1^*, k_2^*, k_3^*$ using silhouette score \cite{ROUSSEEUW198753}. 
    \item[4.] For each target number of subtopics $k^*$,we execute \Cref{alg:tnt-llm-taxonomy-topic} with parameters $B = 200, K=200, N = 30$ using topic-specific initial and update prompts as illustrated in \Cref{fig:subtopic_initial} and \Cref{fig:subtopic_update}. The model used for subtopic discovery is OpenAI-o1, selected for its strong reasoning capabilities. 
    To enforce the desired number of generated subtopics at the start of the iteration, we replace the placeholder ``\{min\_class\_number\_requirement\}'' in \Cref{fig:subtopic_initial} with instruction ``- Generate NO LESS THAN $k^*$ topics.'' . 

    \item [5.]After generating the taxonomy for each $k^*$, we randomly sample 10\% of data instances from the current topic—capped at a maximum of 1000 samples. We then query the o3-mini model, which has strong reasoning ability, using the prompt provided in \Cref{fig:subtopic_assignment}. This yields a set of predicted labels $\{l_1, l_2, \cdots, l_i, \cdots, l_m\}$, along with corresponding relevance scores $\{r_1, r_2, \cdots, r_i, \cdots, r_m\}$ between 0-10, each ranging from 0 to 10. We then compute a quality score for each generated taxonomy using the following equations:

    \begin{equation}
        s_{\text{quality}} = s_{\text{coverage}} + s_{\text{certainty}}
    \end{equation}

    Where $s_{\text{coverage}}$ and $s_{\text{certainty}}$ are defined as: 
    \begin{equation}
        s_{\text{coverage}} = 1.0 - \frac{N_{\text{Undefined}}}{N}
    \end{equation}
    
    where $N_{\text{Undefined}}$ is the number of samples that labeled as ``Undefined'', which is not fit in the taxonomy, and $N$ is the number of data sample labeled for taxonomy validation.
    \begin{equation}
    \begin{aligned}
        p_i &= \frac{r_i}{\sum_{k=0}^m r_k} \\
        H_j &= \frac{\sum_{i=1}^{n}p_i\log_2 p_i}{\log_2m} \\
        s_{\text{certainty}} &=   \frac{\sum_{j=1}^N (1.0 - H_j)} {N}
    \end{aligned}
    \end{equation} 

    We select the best taxonomy generated using $s_{\text{quality}}$. 
 \end{itemize}

\begin{figure*}[htbp]
    \centering
   \begin{tcolorbox}[colframe=borderblue, colback=bggray, left=1mm, right=1mm, top=0.5mm, bottom=0.5mm]
\inputminted[fontsize=\scriptsize, breaklines, breakanywhere, breaksymbolleft={}]{markdown}{appendix/prompts/subtopic_initial_taxonomy_generation.md}
\end{tcolorbox}
    \caption{Initial Taxonomy Generation Prompt For Subtopic}
    \label{fig:subtopic_initial}
\end{figure*}

\begin{figure*}[htbp]
    \centering
   \begin{tcolorbox}[colframe=borderblue, colback=bggray, left=1mm, right=1mm, top=0.5mm, bottom=0.5mm]
\inputminted[fontsize=\scriptsize, breaklines, breakanywhere, breaksymbolleft={}]{markdown}{appendix/prompts/subtopic_taxonomy_update_part1.md}
\end{tcolorbox}
\end{figure*}

\begin{figure*}[htbp]
    \centering
   \begin{tcolorbox}[colframe=borderblue, colback=bggray, left=1mm, right=1mm, top=0.5mm, bottom=0.5mm]
\inputminted[fontsize=\scriptsize, breaklines, breakanywhere, breaksymbolleft={}]{markdown}{appendix/prompts/subtopic_taxonomy_update_part2.md}
\end{tcolorbox}
    \caption{Taxonomy Update Prompt For Subtopic}
    \label{fig:subtopic_update}
\end{figure*}

\begin{figure*}[htbp]
    \centering
   \begin{tcolorbox}[colframe=borderblue, colback=bggray, left=1mm, right=1mm, top=0.5mm, bottom=0.5mm]
\inputminted[fontsize=\scriptsize, breaklines, breakanywhere, breaksymbolleft={}]{markdown}{appendix/prompts/subtopic_assignment.md}
\end{tcolorbox}
    \caption{Subtopic Assignment Prompt}
    \label{fig:subtopic_assignment}
\end{figure*}

\paragraph{Subtopic Label Assignment}
Finally, we label all data samples using the prompt illustrated in \Cref{fig:subtopic_assignment}, with the o3-mini model. For each topic, we select the best-performing taxonomy and use it to annotate all corresponding samples.
    
\subsection{Topic Label Quality Control}

After completing the labeling pipeline, we still observed some false positives upon manual inspection. To address this, we conducted an additional verification step—similar to the initial phase of the subtopic discovery pipeline—by reviewing each data sample alongside its raw conversation, assigned label, and label description, using the o3-mini model and the prompt shown in \Cref{fig:subtopic_verfication}. Following this verification, we removed all samples that lacked a valid label assignment or were assigned the Undefined label at either the topic or subtopic level. This filtering ensured that the final dataset aligned with the discovered taxonomy, ultimately reducing the dataset size to approximately 182k examples.

\begin{figure*}[htbp]
    \centering
   \begin{tcolorbox}[colframe=borderblue, colback=bggray, left=1mm, right=1mm, top=0.5mm, bottom=0.5mm]
\inputminted[fontsize=\scriptsize, breaklines, breakanywhere, breaksymbolleft={}]{markdown}{appendix/prompts/subtopic_verification.md}
\end{tcolorbox}
    \caption{Subtopic Verification Prompt}
    \label{fig:subtopic_verfication}
\end{figure*}

\subsection{Keywords Categorization}

After the labeling process, we observed that certain topics—such as ``Fanfiction and Crossover'' and ``Programming'' contained a disproportionately large number of data samples. To enable more fine-grained question generation, we further categorized the extracted keywords into four semantic types: \textbf{programming language}, \textbf{creative artwork}, \textbf{public figure}, and \textbf{book}. Conversations that do not contain any keywords from these categories are classified as having no keywords.

\subsubsection{LLM Based Aggregation}

Assuming that the same word used by the same user conveys a consistent meaning, we first associate each user’s keyword with its corresponding description, extracted at the beginning of the process. We then employ o3-mini to cluster these raw keywords into semantically coherent groups, corresponding to categories including ``Programming Language'', ``Video Games'', ``Tabletop Games'', ``Manga/Anime'', ``Film'', ``TV Show'', ``Western Cartoon/Comic'', ``Book'', ``Musical'', and ``Public Figure'' , using the prompt illustrated in \Cref{fig:categorize_keywords}.

\begin{figure*}[htbp]
    \centering
   \begin{tcolorbox}[colframe=borderblue, colback=bggray, left=1mm, right=1mm, top=0.5mm, bottom=0.5mm]
\inputminted[fontsize=\scriptsize, breaklines, breakanywhere, breaksymbolleft={}]{markdown}{appendix/prompts/categorize_keywords.md}
\end{tcolorbox}
    \caption{Subtopic Verification Prompt}
    \label{fig:categorize_keywords}
\end{figure*}

\begin{figure*}[htbp]
    \centering
   \begin{tcolorbox}[colframe=borderblue, colback=bggray, left=1mm, right=1mm, top=0.5mm, bottom=0.5mm]
\inputminted[fontsize=\scriptsize, breaklines, breakanywhere, breaksymbolleft={}]{markdown}{appendix/prompts/question_generation.md}
\end{tcolorbox}
    \caption{Question Generation Prompt}
    \label{fig:generate_question}
\end{figure*}

\subsubsection{Rule-based LLM Result Aggregation}

Although o3-mini is prompted to generate the most well-known names for corresponding entities, the model occasionally produces inconsistent outputs, such as ``Pokémon'' vs. ``Pokemon''. These discrepancies are treated as distinct entries in downstream question generation. To address this, we define equivalence between a pair of large language model-generated terms or phrases $(w_a,w_b)$, where $\text{len}(w_a) <= \text{len}(w_b)$ -- based on a set of normalization criteria. Terms are considered equivalent across all keyword types except ``Public Figure'' if they satisfy any of the following conditions after applying string normalization: 

\begin{itemize}
    \item[1.] $w_a$ and $w_b$ are identical. 
    \item[2.] $w_a$ and $w_b$ are identical after removing all stopwords in NLTK English stopwords list. 
    \item[3.] $w_a$ is a prefix of $w_b$ and $w_a$ has more than 2 words. 
    \item[4.] $w_a$ is a suffix of $w_b$ and $w_a$ has more than 2 words.
    \item[5.] $w_a$ is an abbreviation of $w_b$ by concatenating all first letter of $w_b$.
\end{itemize}

For keywords of type ``Public Figure'' only Conditions 1 and 2 are applied due to the higher sensitivity of proper name matching. After normalization, we obtain a dataset with annotated two-level topic hierarchies and keywords spanning the following types: ``Programming Language'', ``Video Games'', ``Tabletop Games'', ``Manga/Anime'', ``Film'', ``TV Show'', ``Western Cartoon/Comic'', ``Book'', ``Musical'', and ``Public Figure''.

\subsection{Question Proposal} 

\paragraph{Attributes Combination} We generate questions through a brute-force search over various combinations and quantities of conditions. The full set of considered conditions is shown in \Cref{tab:att_intro}. Specifically, we enumerate all possible attribute combinations containing 0 to 3 conditions and manually select 73 meaningful combinations that can be naturally expressed in language. The selected combinations are listed in \Cref{tab:data_question_stat}.

\paragraph{Question Proposal Sampling} For each attribute condition and target type combination, we enumerate all possible condition value configurations using MongoDB. For each configuration, we first verify that the number of documents satisfying the condition is at least 50, unless the condition involves the username attribute, in which case the threshold is reduced to 10. This ensures that each generated question is supported by a sufficient number of documents.

Next, we query the database again to check whether the top 3 most frequent target attribute values collectively account for at least 15\% of all occurrences. This constraint prevents cases where the target distribution is overly uniform and lacks distinguishing signals.

All condition-target combinations that pass both checks are then stored in a map, where the key is the top-1 target value and the value is a list of corresponding condition-target combinations. Each list is sorted by the normalized entropy of the target distribution to prioritize more informative combinations.

Finally, we sample from this map in a round-robin manner, ensuring that each value is selected no more than twice. This strategy helps generate the most answerable questions while maintaining diversity across different top-1 target outcomes.

\subsection{Question Generation}
Given a set of condition types, corresponding values, and a target value, we prompt GPT-4.1 to generate natural language questions using the template shown in \Cref{fig:generate_question}.
\begin{figure}[htbp]
    \centering
   \begin{tcolorbox}[colframe=borderblue, colback=bggray, left=1mm, right=1mm, top=0.5mm, bottom=0.5mm]
\inputminted[fontsize=\scriptsize, breaklines, breakanywhere, breaksymbolleft={}]{markdown}{appendix/prompts/qa_prompt.md}
\end{tcolorbox}
    \caption{Question Answering Prompt}
    \label{fig:question_answering}
\end{figure}

Following question generation, we retrieve the top 10 candidate answers for ranking by querying the database. In cases where fewer than 10 valid candidates are available, we supplement them by sampling from the global distribution of values that share the same target type.

Using this procedure, we generated a total of 6,177 questions.

\subsection{Question Quality Control}

We employ o4-mini for final quality control. Specifically, o4-mini is used to rank target candidates under two settings: (1) without any supporting context, and (2) with supporting context provided in the form of either summaries or raw conversations, using the prompting format shown in \Cref{fig:question_answering}.For each instance, we compute the instance-wise NDCG@10 score in the no-context setting, denoted as $s_{\text{no\_context}}$, and define the contextual score as $s_{\text{context}} = \max(s_{\text{raw\_context}}, s_{\text{summary\_context}})$, where $s_{\text{raw\_context}}$ and $s_{\text{summary\_context}}$are scores under raw and summarized contexts, respectively.

To assess statistical significance, we calculate a confidence-based threshold to determine whether a contextual improvement is meaningful over random performance. The threshold is defined as:
\begin{equation}
    s_{\text{threshold}} = \min(1.0, \max(0.0, s_{\text{random}} + z_{0.90} *  s_{\text{std}}))
\end{equation}

where $s_{\text{std}}$ is the standard deviation estimated via a Monte Carlo approach, and $z_{0.90}$ is the 90\%-confidence z-score.We remove any instance that satisfies both of the following conditions:
\begin{itemize}
\item $s_{\text{context}} - s_{\text{no\_context}} \le 0 $
\item $s_{\text{context}} < s_{\text{threshold}} $
\end{itemize}

After filtering, we retain a total of 6,027 valid data samples for downstream evaluation.
