# Supplementary material for: Interactive Training: Feedback-Driven Neural Network Optimization
Source: arXiv:2510.02297 source file (2025-10-02)
Supplement: Supplementary file 2 [file data_profile.tex]

% auto-generated longtable
         % switch from two-column
\section{Data Statistics}
\label{sec:appendix_data_profile}

\subsection{Statistics of Generated Question by Condition and Targets}
\begin{table}[ht]
\centering
\begin{tabularx}{\columnwidth}{>{\raggedright\arraybackslash}X l r}
\toprule
Condition & Target & Count \\
\midrule
 \multicolumn{3}{c}{0 Condition}   \\
\midrule
none & topic & 1 \\ 
none & loc & 1 \\ 
none & lang & 1 \\ 
\midrule
 \multicolumn{3}{c}{1 Condition}   \\
\midrule
user & keywords & 370 \\ 
user & time & 100 \\ 
keywords & user & 96 \\ 
user & lang & 60 \\ 
user & topic & 54 \\ 
time & user & 39 \\ 
topic & subtopic & 26 \\ 
loc & topic & 20 \\ 
loc & keywords & 17 \\ 
lang & topic & 9 \\ 
time & topic & 6 \\ 
time & keywords & 6 \\ 
topic & loc & 6 \\ 
topic & user & 6 \\ 
topic & lang & 4 \\ 
topic & keywords & 4 \\ 
time & lang & 4 \\ 
lang & keywords & 1 \\ 
\midrule
 \multicolumn{3}{c}{2 Conditions}   \\
\midrule
user, topic & subtopic & 199 \\ 
user, topic & keywords & 185 \\ 
user, user & subtopic & 141 \\ 
user, topic & time & 114 \\ 
topic, lang & subtopic & 100 \\ 
time, topic & user & 98 \\ 
time, topic & subtopic & 98 \\ 
topic, lang & user & 98 \\ 
topic, loc & time & 97 \\ 
topic, keywords & user & 97 \\ 
\bottomrule
\end{tabularx}
\caption{Question Type Statistics}
\label{tab:data_question_stat}
\end{table}

\begin{table}[!t]
\centering
\begin{tabularx}{\columnwidth}{>{\raggedright\arraybackslash}X l r}
\toprule
Condition & Target & Count \\
\midrule
topic, loc & subtopic & 96 \\ 
topic, keywords & time & 96 \\ 
time, user & keywords & 94 \\ 
topic, subtopic & user & 93 \\ 
subtopic, subtopic & user & 93 \\ 
topic, loc & keywords & 82 \\ 
topic, lang & time & 74 \\ 
time, topic & loc & 60 \\
topic, subtopic & keywords & 55 \\ 
topic, topic & user & 55 \\ 
time, user & topic & 53 \\ 
user, user & topic & 53 \\ 
time, topic & keywords & 49 \\ 
topic, subtopic & loc & 39 \\ 
time, loc & topic & 34 \\ 
time, lang & topic & 31 \\ 
topic, lang & keywords & 27 \\ 
time, topic & lang & 15 \\ 
topic, subtopic & lang & 13 \\ 
topic, loc & user & 10 \\ 
\midrule
 \multicolumn{3}{c}{3 Conditions}   \\
\midrule
loc, topic, subtopic & user & 287 \\ 
lang, topic, subtopic & user & 284 \\ 
user, topic, subtopic & keywords & 276 \\ 
time, loc, topic & user & 199 \\ 
time, topic, subtopic & keywords & 175 \\ 
user, user, user & subtopic & 132 \\ 
user, topic, keywords & time & 114 \\ 
time, topic, keywords & user & 100 \\ 
time, loc, topic & subtopic & 100 \\ 
time, user, topic & subtopic & 100 \\ 
loc, topic, keywords & user & 99 \\ 
user, topic, subtopic & time & 98 \\ 
user, topic, keywords & subtopic & 98 \\ 
loc, topic, keywords & time & 98 \\ 
lang, topic, keywords & time & 98 \\ 
time, topic, subtopic & user & 97 \\ 
lang, topic, keywords & user & 96 \\ 
topic, subtopic, keywords & user & 94 \\ 
loc, topic, subtopic & keywords & 93 \\ 
lang, topic, subtopic & keywords & 82 \\ 
time, topic, subtopic & loc & 76 \\ 
user, user, user & topic & 51 \\ 

\bottomrule
\end{tabularx}
\end{table}

%\onecolumn    
\subsection{Language Distribution}
We provide a statistics of all language involved in the conversations in \Cref{tab:all_language_statistics}.
\begin{table*}[ht]
\centering

\begin{tabular}{lrlrlrlr}
\toprule
\textbf{Language} & \textbf{Count} & \textbf{Language} & \textbf{Count} & \textbf{Language} & \textbf{Count} & \textbf{Language} & \textbf{Count} \\
\midrule
English & 124,646 & Spanish & 4,193 & Italian & 744 & Polish & 527 \\
Russian & 22,877 & Portuguese & 3,532 & Korean & 605 & Vietnamese & 463 \\
Chinese & 6,434 & Turkish & 1,408 & Indonesian & 566 & Ukrainian & 406 \\
French & 4,782 & Latin & 1,239 & Dutch & 549 & Other & 1,824 \\
German & 4,487 & Arabic & 863 & Tagalog & 537 & & \\
\bottomrule
\end{tabular}
\caption{Language Statistics in Conversations}
\label{tab:all_language_statistics}
\end{table*}

\subsection{Keywords Cloud}
To illustrate the result of keywords categorization, we build a keywords cloud in \Cref{fig:keyword_cloud}
\begin{figure*}[h]
    \centering
    \includegraphics[width=\linewidth]{figures/wordcloud.pdf}
    \caption{Word Cloud of All Keywords}
    \label{fig:keyword_cloud}
\end{figure*}
\subsection{Topic and Subtopic overview}
\clearpage

\small 
% auto-generated longtable
\onecolumn
\begin{longtable}{llr}
\caption{Topic Taxonomy in WildChat-AQA}\label{tab:topic_taxonomy_full}\\
\toprule
\textbf{Parent Topic} & \textbf{Sub-topic} & \textbf{Count}\\
\midrule
\endfirsthead
\multicolumn{3}{c}{\textit{Topic Taxonomy in WildChat-AQA (continued)}}\\
\midrule
\textbf{Parent Topic} & \textbf{Sub-topic} & \textbf{Count}\\
\midrule
\endhead
\midrule
\multicolumn{3}{r}{\textit{Continued on next page}}\\
\endfoot
\midrule
\endlastfoot
\multirow{13}{*}{Creative Writing and Fiction} & Dialogue \& Scripted Scenes & 25421\\
 & Fanfiction \& Universe Crossovers & 20323\\
 & Extended Narrative Prose & 19771\\
 & Humorous \& Satirical Narratives & 11901\\
 & Erotic \& Sensual Narratives & 8304\\
 & World-Building \& Adventure Narratives & 6470\\
 & Creative Naming \& Prompt Generation & 4388\\
 & Sports \& Competition Narratives & 3370\\
 & Transformation \& Identity Narratives & 3283\\
 & Character Profiles \& Descriptions & 2025\\
 & Fictional News \& Media Formats & 1912\\
 & Poetic \& Lyric Composition & 1608\\
 & Interactive \& Roleplaying Narratives & 827\\
\midrule
\multirow{16}{*}{Law, Regulation and Criminal Justice} & Violent Crimes & 630\\
 & Regulatory Compliance and Licensing & 454\\
 & Civil Litigation and Consumer Protection & 284\\
 & Employment and Labor Law & 198\\
 & Sexual Crimes & 183\\
 & Intellectual Property and Copyright & 163\\
 & Financial, Fraud, and Cyber Offenses & 142\\
 & Robbery, Theft, and Property Offenses & 130\\
 & Judicial Process and Court Administration & 117\\
 & Constitutional Rights and Civil Liberties & 81\\
 & Terrorism, War Crimes, Treason, and Political Violence & 68\\
 & Corruption and Abuse of Power & 64\\
 & Public Order Offenses & 54\\
 & Immigration and Border Control & 51\\
 & Drug-Related Offenses & 50\\
 & Family and Marital Law & 48\\
\midrule
\multirow{13}{*}{Entertainment, Games, and Media} & Fanfiction \& Crossovers & 25629\\
 & Original Fiction \& Scripts & 4834\\
 & NSFW \& Explicit Scenes & 3717\\
 & Live-Action Film \& TV & 2963\\
 & Western Animation \& Comics & 2048\\
 & Gaming Story \& Lore & 1895\\
 & Celebrity \& Pop Culture & 1882\\
 & Gaming Mechanics \& Tech & 1660\\
 & Music \& Stage & 1651\\
 & Sports, eSports, \& Pro Wrestling & 1557\\
 & Anime \& Manga & 1552\\
 & Production \& Broadcasting & 1044\\
 & Tabletop \& TTRPG & 804\\
\midrule
\multirow{21}{*}{Software, Programming and Computer Science} & Programming & 17413\\
 & Web Development & 3603\\
 & AI and Machine Learning & 2787\\
 & Cybersecurity & 1930\\
 & Game Development, Design, and Modding & 1737\\
 & Databases and Queries & 1724\\
 & Operating Systems and Administration & 1414\\
 & Productivity and Desktop Software & 1215\\
 & Computer Networking & 1176\\
 & DevOps and Cloud & 1083\\
 & Data Analysis, Visualization and Business Intelligence & 1031\\
 & Mobile Development and Mobile Apps & 972\\
 & Computer Graphics & 740\\
 & Computer Science Theory & 612\\
 & Computer Hardware, Architecture, and Peripherals & 576\\
 & Software Architecture and Software System Design & 438\\
 & Testing and Quality Assurance & 350\\
 & Blockchain and Cryptocurrency & 336\\
 & Embedding Systems and IoT & 286\\
 & Human Computer Interaction & 184\\
 & Software Development Methodology and Project Management & 165\\
\midrule
\multirow{14}{*}{Science, Mathematics and Logical Reasoning} & Physics: Mechanics, Thermodynamics, and Fields & 1877\\
 & Basic Arithmetic and Numbers & 1376\\
 & Organismal Biology and Evolution & 1360\\
 & General Chemistry and Reactions & 1339\\
 & Cellular and Medical Sciences & 1239\\
 & Astronomy and Astrophysics & 1130\\
 & Earth Science and Environment & 1031\\
 & Statistics and Probability & 912\\
 & Algebra and Vectors & 833\\
 & Logic and Puzzles & 795\\
 & Geometry and Trigonometry & 724\\
 & Computational Science and Modeling & 610\\
 & Calculus and Higher Mathematics & 505\\
 & Materials, Engineering, and Technology & 363\\
\midrule
\multirow{20}{*}{Personal Advice and Support} & Navigating Romance and Dating & 464\\
 & Enhancing Personal Growth and Discipline & 286\\
 & Building Communication and Social Skills & 164\\
 & Offering Emotional Support and Love & 137\\
 & Navigating Sexual Intimacy, Consent, and Well-Being & 128\\
 & Supporting Mental Health and Well-Being & 111\\
 & Guiding Family, Parenting, and Caregiving & 99\\
 & Boosting Self-Confidence and Esteem & 81\\
 & Handling Career and Workplace Challenges & 73\\
 & Exploring Personal Values and Choices & 70\\
 & Seeking Apologies, Forgiveness, and Trust & 65\\
 & Addressing Financial Management and Housing & 47\\
 & Improving Physical Health and Body Image & 47\\
 & Managing Unwanted Contact and Boundaries & 38\\
 & Seeking Legal Guidance and Protective Measures & 34\\
 & Embracing Identity and Lifestyle Transitions & 32\\
 & Recovering from Breakups and Heartache & 32\\
 & Handling Emergencies, Threats, or Crises & 30\\
 & Overcoming Addictions and Harmful Habits & 19\\
 & Coping with Grief and Loss & 15\\
\midrule
\multirow{13}{*}{Business, Commerce and Finance} & Digital Marketing \& Social Media & 4010\\
 & Investments \& Financial Markets & 934\\
 & Business Operations \& Quality Management & 914\\
 & Accounting \& Financial Reporting & 891\\
 & Economic Trends \& Macro Outlook & 739\\
 & Corporate Governance \& Leadership & 492\\
 & Customer Service \& Complaints & 460\\
 & Legal \& Regulatory Compliance & 435\\
 & Supply Chain \& Logistics & 426\\
 & Wholesale \& B2B Distribution & 404\\
 & Banking \& Monetary Policies & 402\\
 & Careers \& Professional Development & 373\\
 & Entrepreneurship \& Startups & 356\\
\midrule
\multirow{26}{*}{History and Culture} & Modern and Contemporary History (19th Century–Present) & 1407\\
 & Conflicts and Wars & 1088\\
 & Medieval Europe & 716\\
 & Philosophy and Political Ideologies & 624\\
 & Art, Architecture, and Heritage & 616\\
 & Religion and Theology & 513\\
 & Traditions, Customs, and Rituals & 395\\
 & Popular Culture and Mass Media & 388\\
 & Pre-Modern East Asia & 386\\
 & Colonialism, Imperialism, and Independence & 343\\
 & Ancient Non-Classical Civilizations & 322\\
 & Classical Rome & 269\\
 & Diplomacy and Treaties & 251\\
 & Language and Literature & 240\\
 & Archaeology and Ancient Technologies & 217\\
 & Sports and Leisure & 197\\
 & Civil Rights and Social Justice & 192\\
 & Ancient Greece and Hellenic Culture & 174\\
 & Legal Systems and Codes & 172\\
 & Social Hierarchies and Slavery & 170\\
 & Myths and Folklore & 166\\
 & Gender and Women’s History & 166\\
 & Indigenous Peoples & 157\\
 & Science and Medicine & 154\\
 & Islamic and Middle Eastern Empires & 119\\
 & Exploration and Discoveries & 100\\
\midrule
\multirow{22}{*}{Lifestyle and Hobbies} & Exploring fashion and accessories & 204\\
 & Hair and Personal Grooming & 189\\
 & Beauty, makeup, and self-care & 110\\
 & Health, sports, and active living & 107\\
 & Minimalist living and conscious habits & 95\\
 & Personal expression, identity, and body positivity & 81\\
 & Creative crafts and DIY projects & 67\\
 & Outdoor Recreation and Camping & 61\\
 & Relationships, family, and social bonding & 59\\
 & Pets, animals, and responsible care & 46\\
 & Spirituality, meditation, and mindfulness & 45\\
 & Music, dance, and performing arts & 43\\
 & Games, collecting, and playful hobbies & 42\\
 & Social events, parties, and gatherings & 40\\
 & Costumes and cosplay & 37\\
 & Cooking, baking, and culinary hobbies & 31\\
 & Productivity and time management & 30\\
 & Travel, tourism, and new adventures & 24\\
 & Digital lifestyle and social media presence & 24\\
 & Seasonal festivities and holiday decorating & 12\\
 & Gardening and horticulture & 7\\
 & Home organization and interior comfort & 6\\
\midrule
\multirow{20}{*}{Academic Resource, Education and Learning} & Academic Research, Methods, and Presentation & 801\\
 & Curriculum and Course Development & 697\\
 & STEM and Technical Education & 428\\
 & Teaching Strategies and Pedagogical Tools & 423\\
 & Health and Medical Education & 326\\
 & Technology and AI Integration in Education & 296\\
 & Professional and Vocational Training & 248\\
 & Educational Policy and Leadership & 195\\
 & University Admissions and Scholarship Guidance & 157\\
 & Language Learning and Translation & 135\\
 & Memory, Study, and Exam Strategies & 118\\
 & Creative Arts and Literature in Education & 110\\
 & Early Childhood Education and Development & 104\\
 & Special Education and Inclusive Learning & 66\\
 & Socio-Emotional Learning and Wellbeing & 60\\
 & Environmental and Social Education & 43\\
 & Academic Ethics and Publication Guidelines & 34\\
 & Parental Engagement and Child Education & 34\\
 & Classroom Management and Student Engagement & 25\\
 & Undefined & 2\\
\midrule
\multirow{24}{*}{Psychology, Mental Health and Emotional Support} & Communication Skills \& Empathy & 211\\
 & Child \& Adolescent Mental Health & 199\\
 & Relationship \& Interpersonal Challenges & 181\\
 & Stress, Coping Strategies \& Resilience & 158\\
 & Mood Disorders (Depression \& Bipolar) & 155\\
 & Anxiety, Panic \& Phobias & 112\\
 & Psychological Theories \& Historical Perspectives & 109\\
 & Therapy \& Counseling Methods & 103\\
 & Sexual Orientation, Gender \& Sexual Behaviors & 102\\
 & Trauma \& PTSD & 99\\
 & Emotional Support for Crises \& Suicidal Ideation & 97\\
 & Self-esteem \& Self-sabotage & 95\\
 & Neurodevelopmental Disorders (ADHD, Autism, etc.) & 90\\
 & Addiction \& Substance Use & 69\\
 & Abuse, Violence \& Bullying & 67\\
 & Grief \& Loss & 54\\
 & Personality Disorders & 42\\
 & Schizophrenia \& Psychotic Symptoms & 38\\
 & Social \& Cultural Factors in Mental Health & 37\\
 & Sleep \& Dream Analysis & 36\\
 & Dissociative Disorders \& Maladaptive Daydreaming & 33\\
 & Medication \& Pharmacological Discussions & 28\\
 & Eating \& Body Image Disorders & 25\\
 & Obsessive \& Compulsive Disorders & 16\\
\midrule
\multirow{20}{*}{Interactive Activities with AI Chatbots} & Explicit or Sexual Roleplay & 1023\\
 & Developer Mode or Policy-Breaking Requests & 456\\
 & Interactive Storytelling with User Control & 380\\
 & Comedic or Vulgar Roleplay & 256\\
 & Flirty or Romantic Scenarios & 217\\
 & Childlike or Energetic Roleplay & 188\\
 & Game or Puzzle Interactions & 162\\
 & Roleplay with Personal or Close Relationships & 112\\
 & Fantasy or Mythical Adventures & 101\\
 & Roleplay with Non-Human Traits & 78\\
 & Action or Combat-Based Roleplay & 77\\
 & Testing Chatbot’s Memory or Logic & 68\\
 & Roleplay with Theatrical or Literary Flair & 60\\
 & Roleplay with Real-World Professions & 49\\
 & Minimalistic or Symbolic Responses Only & 44\\
 & Roleplay with Custom Machinery or System Simulation & 43\\
 & Roleplay with Worship or Devotion & 37\\
 & Roleplay with Social or Political Themes & 29\\
 & Roleplay as Rebels or Criminals & 27\\
 & Hypnosis or Therapeutic Roleplay & 7\\
\midrule
\multirow{9}{*}{Linguistics, Language and Translation} & Rewriting and Paraphrasing & 8331\\
 & Translation & 7997\\
 & Vocabulary and Terminology & 2586\\
 & Proof Reading and Grammar Correction & 2102\\
 & Linguistic Analysis & 1099\\
 & Summarization & 779\\
 & Language Learning Assistance & 503\\
 & Phonetics and Pronunciation & 464\\
 & Information Extraction & 391\\
\midrule
\multirow{7}{*}{Social Issues, Politics and Governance} & Domestic Governance \& Public Policy & 1334\\
 & Political Theories \& Ideological Debates & 1231\\
 & International Relations \& Geopolitics & 1190\\
 & Social Justice, Identity \& Cultural Norms & 1009\\
 & Political Leadership \& Electoral Dynamics & 742\\
 & National Security \& Crisis Management & 543\\
 & Economic Policy \& Regulation & 366\\
\midrule
\multirow{27}{*}{Medicine and Health} & Orthopedics and Musculoskeletal Health & 467\\
 & Nutrition and Dietary Supplements & 466\\
 & Infectious Diseases and Vaccines & 385\\
 & Rehabilitation and Recovery & 384\\
 & Pharmacology and Medication Safety & 378\\
 & Eye, ENT, and Respiratory Conditions & 376\\
 & Surgery and Emergency Care & 341\\
 & Mental Health and Wellbeing & 328\\
 & Reproductive Health and Childbirth & 313\\
 & Digestive, Metabolic, and Endocrine Disorders & 304\\
 & Sexual Health and Function & 243\\
 & Healthcare Systems and Public Health & 238\\
 & Neurology and Nervous System Disorders & 212\\
 & Dermatology and Skin Care & 201\\
 & Diagnostic Tests and Imaging & 190\\
 & Cardiovascular Diseases and Hypertension & 181\\
 & Exercise, Fasting, and Weight Control & 177\\
 & Pediatrics and Child Health & 169\\
 & Preventive Medicine and Wellness & 152\\
 & Cancer and Oncological Care & 141\\
 & Medical Technology and Telemedicine & 109\\
 & Oral Health and Dentistry & 103\\
 & Substance Use and Addiction & 96\\
 & Allergies and Immune Conditions & 88\\
 & Occupational and Environmental Health & 80\\
 & Genetics and Rare Conditions & 76\\
 & Veterinary Medicine and Animal Health & 42\\
\midrule
\multirow{32}{*}{Technology, Engineering and Industry} & Mechanical Engineering and Manufacturing & 678\\
 & Electrical and Electronics Design & 418\\
 & Materials Science and Engineering & 405\\
 & Aerospace and Space Exploration & 381\\
 & Consumer Electronics and Gadgets & 364\\
 & Big Data, IoT, and Smart Systems & 310\\
 & Blockchain and Decentralized Tech & 305\\
 & Networking, Telecommunications, and Cybersecurity & 287\\
 & Civil Engineering and Infrastructure & 278\\
 & Automotive Engineering and Vehicle Technology & 257\\
 & AI and Machine Learning & 251\\
 & VR, AR, and XR Solutions & 245\\
 & Industrial Safety and Compliance & 220\\
 & Robotics, Drones, and Mechatronics & 203\\
 & Military and Defense Technology & 185\\
 & Energy and Sustainable Manufacturing & 156\\
 & Cloud, Virtualization, and Enterprise Platforms & 131\\
 & Supply Chain and Logistics Management & 115\\
 & Software Development and Web Frameworks & 108\\
 & Quantum and High-Performance Computing & 101\\
 & Agricultural Engineering and Food Industry & 84\\
 & Digital Media, Broadcasting, and Streaming & 75\\
 & Hardware Innovation and CPU/GPU Development & 68\\
 & HCI, UI/UX, and Interactive Tech & 67\\
 & Marine and Offshore Engineering & 62\\
 & Data Storage and Retention & 61\\
 & Engineering Education and STEM Training & 55\\
 & Biomedical, Biotech, and Wearables & 55\\
 & Gaming Technology and eSports & 46\\
 & Industrial Digitalization and Change Management & 37\\
 & Product Design and Industrial Innovation & 29\\
 & 3D Printing and Additive Manufacturing & 16\\
\midrule
\multirow{15}{*}{General Digital Support} & AI Capabilities & 472\\
 & AI Limitations & 397\\
 & AI Identity, Version, and Origins & 161\\
 & Correcting or Revising AI Responses & 61\\
 & Technical Guidance: External Apps and Websites & 57\\
 & AI Emotions or Opinions & 48\\
 & Creative Writing & 38\\
 & Official Links or Verification & 33\\
 & Coding Tasks & 29\\
 & Technical Guidance: Phones and Software & 24\\
 & Email and Account Management & 19\\
 & Comparison with Other AI Systems & 18\\
 & Education or Research Use & 17\\
 & Search and Browsing Advice & 10\\
 & Payment or Subscription & 5\\
\midrule
\multirow{5}{*}{Food, Cooking and Nutrition} & Nutritional Guidance \& Diet Planning & 569\\
 & Recipes \& Cooking Techniques & 518\\
 & Ingredient Selection \& Quality & 218\\
 & Culinary Culture \& Dining Experience & 166\\
 & Food Safety \& Storage & 76\\
\midrule
\multirow{13}{*}{Art and Design} & Product \& Merchandise Design & 1086\\
 & AI-Generated Art \& Prompt Engineering & 585\\
 & Digital Media \& Advertising Design & 492\\
 & Color Theory \& Visual Composition & 407\\
 & Character \& Animation Design & 290\\
 & Art History \& Critique & 270\\
 & Editorial \& Commercial Illustration & 262\\
 & Fashion \& Costume Design & 252\\
 & Logo \& Branding Design & 213\\
 & Educational \& Children's Art & 204\\
 & Architectural \& Environmental Design & 192\\
 & Digital Art \& Software Techniques & 132\\
 & Traditional \& Manual Art Techniques & 116\\
\midrule
\multirow{10}{*}{Religion, Mythology and Spirituality} & Biblical and Scriptural Narratives & 981\\
 & Islamic Sacred Narratives & 363\\
 & Classical Mythology Narratives & 356\\
 & Eastern Sacred Narratives & 243\\
 & Modern Esoteric and Occult Spirituality & 188\\
 & Religion, Society, and Cultural Critique & 178\\
 & Astrological and Divinatory Traditions & 169\\
 & Folk and Indigenous Myth Narratives & 164\\
 & Norse and Germanic Mythological Narratives & 44\\
 & Ancient Near Eastern and Persian Narratives & 31\\
\midrule
\multirow{4}{*}{Literature and Book Analysis} & Narrative and Prose Analysis & 1482\\
 & Poetry and Versified Analysis & 427\\
 & Literary Guidance and Recommendations & 355\\
 & Advanced Literary Criticism & 43\\
\midrule
\multirow{18}{*}{Philosophy and Ethics} & Epistemology, Logic, and Fallacies & 349\\
 & Law, Governance, and Political Philosophy & 341\\
 & Mind, Consciousness, and Reality & 303\\
 & Religion, Theology, and Faith Traditions & 299\\
 & Existentialism, Death, and Meaning & 176\\
 & Moral Theories, Virtue, and Character Development & 171\\
 & Moral Speech and Expression & 146\\
 & Critical Theory and Postmodernism & 133\\
 & Consent, Power, and Manipulation & 104\\
 & Cultural Norms and Social Ethics & 100\\
 & Aesthetics and Artistic Philosophy & 91\\
 & Ethics in AI and Future Technologies & 90\\
 & Professional Ethics and Duty & 81\\
 & Markets, Capitalism, and Economic Fairness & 43\\
 & Bioethics, Medicine, and Life Origins & 42\\
 & Morality Toward Animals & 40\\
 & Love, Relationships, and Emotional Ethics & 28\\
 & Environmental Ethics and Sustainability & 19\\
\midrule
\multirow{19}{*}{Sports and Athletics} & NCAA College Football & 1012\\
 & Motorsport & 607\\
 & NBA Basketball & 604\\
 & NCAA College Basketball & 549\\
 & Global Soccer & 538\\
 & Fictional or Hypothetical Scenarios & 451\\
 & Professional American Football & 313\\
 & General or Cross-Sport Training \& Fitness & 218\\
 & Professional Wrestling & 146\\
 & Baseball & 68\\
 & Combat Sports & 64\\
 & Cricket & 60\\
 & Cycling (Races \& Gear) & 59\\
 & Ice Hockey & 25\\
 & Tennis and Other Racket Sports & 18\\
 & Rugby & 14\\
 & Gymnastics \& Swimming & 7\\
 & Volleyball & 3\\
 & Golf & 2\\
\midrule
\multirow{33}{*}{Environment, Ecology and Sustainability} & Climate Change Causes, Impacts, and Adaptation & 140\\
 & Biodiversity Conservation and Wildlife Protection & 119\\
 & Greenhouse Gas Emissions and Carbon Management & 117\\
 & Pollution (Air, Water, Soil) and Remediation & 102\\
 & Waste Management and Circular Economy & 101\\
 & Environmental Policies, Laws, and Regulations & 82\\
 & Sustainable Energy and Energy Transition & 74\\
 & Green Industry, Corporate Sustainability, and Innovation & 72\\
 & Water Resource Management and Conservation & 67\\
 & Ecological Economics and Sustainable Development & 66\\
 & Environmental Education and Public Awareness & 45\\
 & Deforestation, Reforestation, and Sustainable Forestry & 43\\
 & Environmental Monitoring, Data Analysis, and Reporting & 40\\
 & Sustainable Lifestyles and Consumer Choices & 39\\
 & Sustainable Packaging, Recycling, and Plastics Reduction & 37\\
 & Sustainable Agriculture and Food Systems & 35\\
 & Marine and Coastal Conservation & 33\\
 & Sustainable Cities and Urban Development & 33\\
 & Ecological Restoration and Ecosystem Management & 33\\
 & Digital Technologies and Sustainability & 32\\
 & Sustainable Architecture and Construction & 26\\
 & Sustainable Transportation and Mobility & 23\\
 & Soil Health and Land Use Management & 22\\
 & Environmental Disaster Preparedness and Risk Reduction & 20\\
 & Carbon Markets and Climate Finance & 19\\
 & Eco-friendly Materials and Green Design & 17\\
 & Community-based Conservation and Participation & 15\\
 & Climate Negotiations and International Agreements & 12\\
 & Protected Areas and Natural Heritage Sites & 12\\
 & Environmental and Climate Justice & 11\\
 & Conservation Technology and Innovation & 6\\
 & Environmental Impact Assessment and Life Cycle Analysis & 5\\
 & Sustainable Tourism and Ecotourism & 3\\
\midrule
\multirow{10}{*}{Travel and Tourism} & Cultural, Heritage \& City Experiences & 126\\
 & Transport \& Logistics & 87\\
 & Travel Itineraries \& Trip Planning & 65\\
 & Accommodation \& Lodging & 54\\
 & Tourism Industry, Policy \& Market & 49\\
 & Culinary \& Dining & 40\\
 & Visa \& Travel Documentation & 40\\
 & Beach, Coastal \& Cruise Tourism & 37\\
 & Entertainment \& Nightlife & 28\\
 & Adventure \& Outdoor Activities & 25\\
\midrule
\multirow{15}{*}{Professional Development and Career Advice} & Cover Letters \& SOPs & 270\\
 & Resume \& CV Enhancement & 233\\
 & Workplace Culture \& Dynamics & 132\\
 & Skill Development \& Advanced Education & 128\\
 & Leadership \& Team Management & 106\\
 & Salary \& Compensation Guidance & 96\\
 & Recruitment \& Talent Acquisition & 96\\
 & Industry-Specific Career Advice & 75\\
 & LinkedIn \& Personal Branding & 69\\
 & Job Search \& Networking Strategies & 60\\
 & Career Transitions \& Upskilling & 60\\
 & Negotiation \& Employment Contracts & 42\\
 & Interview Preparation \& Techniques & 31\\
 & Employment Documentation \& Verification & 31\\
 & Freelancing \& Entrepreneurship & 19\\
\midrule
\multirow{17}{*}{Home and Household} & Gardening: Planting \& General Care & 140\\
 & Gardening: Soil \& Fertilization & 128\\
 & Fruit \& Berry Cultivation & 107\\
 & Home Fixtures \& Materials & 83\\
 & Gardening: Pest \& Disease Management & 75\\
 & Interior Design \& Decoration & 60\\
 & Home Maintenance \& Appliance Repair & 54\\
 & Laundry \& Fabric Care & 36\\
 & DIY Tools \& Household Projects & 31\\
 & Household Cleaning \& Stain Removal & 27\\
 & Outdoor Landscaping \& Mulching & 24\\
 & Eco-Friendly \& Sustainable Practices & 15\\
 & Household Safety \& Security & 14\\
 & Real Estate \& Tenancy & 13\\
 & Household Management \& Lifestyle & 13\\
 & Home Organization \& Storage Solutions & 8\\
 & Household Pets \& Animal Care & 5\\
\end{longtable}
\twocolumn
\clearpage

\normalsize            % restore size if you changed it
%\twocolumn 
