# Supplementary material for: Interactive Training: Feedback-Driven Neural Network Optimization
Source: arXiv:2510.02297 source file (2025-10-02)
Supplement: Supplementary file 3 [file data_visualization_and_implementation.tex]

\begin{figure*}[!t]
    \centering
    \includegraphics[width=\linewidth]{figures/visualization/demo.png}
    \caption{Data Visualization Demo Overview}
    \label{fig:demo-main}
\end{figure*}

\vspace{1em} % optional spacing

\section{Data Visualization Demonstration}

We developed an interactive data visualization interface using React.js and Next.js for the frontend, and FastAPI for the backend implementation. MongoDB serves as the database system. An overview of the interface is shown in \Cref{fig:demo-main}. Users can filter generated questions using a configurable question filter, as illustrated in \Cref{fig:demo-filter}.

\begin{figure}[h]
    \centering
    \includegraphics[width=0.95\linewidth]{figures/visualization/filter_bar.png}
    \caption{Question filter attributes of different conditions and targets.}
    \label{fig:demo-filter}
\end{figure}

The filtering mechanism allows users to select one or more attributes for both the condition and target fields to retrieve relevant questions. For instance, the filters ``user\_pair'' and ``user\_triplet'' refer to questions based on common interests between two or three users, respectively. Similarly, ``joint\_topic'' and ``joint\_subtopic'' denote filters that select conversations involving shared topics or subtopics.

\begin{figure}[h]
    \centering
    \includegraphics[width=0.95\linewidth]{figures/visualization/token_time_distribution.png}
    \caption{Context conversation and token count and distribution of conversation over time. }
    \label{fig:demo-filter2}
\end{figure}

\begin{figure}[h]
    \centering
    \includegraphics[width=0.95\linewidth]{figures/visualization/distribution_display.png}
    \caption{Distribution of topics}
    \label{fig:demo-filter3}
\end{figure}

For each question, the interface displays the number of supporting dialogues and their associated token counts. Additional distributions—such as raw keywords, aggregated keywords, language, topic, location, and user identity—are visualized to facilitate deeper insights.

\begin{figure*}[ht]
    \centering
    \includegraphics[width=0.95\linewidth]{figures/visualization/detail_display.png}
    \caption{Dialogue Detail Display}
    \label{fig:demo-main2}
\end{figure*}

Users can also explore the ``DIALOGUES'' panel to view all conversation excerpts that support a particular question. Each dialogue entry includes detailed metadata: username, timestamp, topic, subtopic, generated summary, raw extracted keywords, and aggregated keywords. This comprehensive display allows users to audit or explore the basis of each proposed question in context.

\section{Experiment Implementation Details}

\label{appendix:implementation_details}

We employed MongoDB v8.0.4 for question proposal generation and ground-truth-based retrieval. All retrieval experiments utilizing BM25 and dense kNN methods were conducted using Elasticsearch v8.18. Training and inference for open-source models were carried out on a range of GPUs, including the NVIDIA RTX A6000 Ada, NVIDIA H100, and NVIDIA H200, depending on availability.

For all embedding-based dense retrieval experiments, the questions, generated queries, documents, and summaries were encoded using the OpenAI \texttt{text-embedding-3-large} model, which produces 3072-dimensional vectors.

For fine-tuning experiments with Qwen3-8B, we used the HuggingFace Transformers library \cite{wolf2020huggingfacestransformersstateoftheartnatural}, version 4.51.3, training on the full conversation dataset with a peak learning rate of $1 \times 10^{-5}$, a batch size of 8, and a linear learning rate decay schedule.

For inference with open-source models, we utilized vLLM v0.8.5.post1. The sampling hyperparameters used during inference are detailed in \Cref{tab:inference_param}.

\begin{table}[h]
    \centering
    \small
    \begin{tabular}{lccc}
        \toprule
        Model Name      & top\_p    & top\_k    &   temperature \\
        \midrule
        Gemma3-4B       & 0.95      &  64       &   1.0         \\
        Qwen3-8B        & 0.8       &  20       &   0.7         \\
        Qwen3-8B-Think  & 0.95      &  20       &   0.6         \\
        Qwen3-32B       & 0.8       &  20       &   0.7         \\
        Qwen3-32B Think & 0.95      &  20       &   0.6         \\
        GPT-4.1-mini    & 1.0       & -         &   1.0         \\
        o4-mini         & -         & -         &   -           \\
        \bottomrule
    \end{tabular}
    \caption{Model sampling hyper-parameter}
    \label{tab:inference_param}
\end{table}

For query generation in \textbf{PROBE}, we use GPT-4.1-mini as query and filter generator with top\_p = 0.5 and top\_k = 0.5.
