# Supplementary material for: Interactive Training: Feedback-Driven Neural Network Optimization
Source: arXiv:2510.02297 source file (2025-10-02)
Supplement: Supplementary file 4 [file related_works.tex]

\section{Related Works}

\paragraph{Question Answering} Question answering typically involves a diverse range of perspectives. Datasets such as TriviaQA \cite{joshi-etal-2017-triviaqa}, RACE \cite{lai-etal-2017-race}, HotPotQA \cite{yang2018hotpotqa}, Natural Questions \cite{kwiatkowski-etal-2019-natural}, MuSiQue \cite{trivedi-etal-2022-musique}, 2Wiki \cite{ho-etal-2020-constructing}, PopQA \cite{mallen2023trustlanguagemodelsinvestigating}, and MultiHop-RAG \cite{tang2024multihopragbenchmarkingretrievalaugmentedgeneration} focus on \textbf{local information}, where answers can be derived from one or several documents.
In contrast, other benchmarks such as MMLU \cite{hendrycks2021measuring}, MATH \cite{hendrycksmath2021}, GSM8K \cite{cobbe2021gsm8k}, and Big-Bench \cite{srivastava2023beyond} emphasize science, technology, engineering, mathematics, and logical reasoning. These primarily evaluate models' world knowledge and reasoning capabilities but lack a benchmark for understanding large-scale datasets and deriving high-level insights.
Recent works such as GraphRAG \cite{edge2025localglobalgraphrag} address the long-context challenge by extracting entities and relationships from extended text data and constructing graph structures to answer questions.

\paragraph{Long Context Retrieval Augmented Generation}  \cite{NEURIPS2020_6b493230} has emerged as a prominent approach for enhancing the performance of large language models (LLMs) on knowledge-intensive tasks while also mitigating hallucinations. Recently, advances in computational capabilities have spurred interest in extending RAG to support very long contexts. Several studies—such as those by \citet{jiang2024longragenhancingretrievalaugmentedgeneration}, \citet{zhao-etal-2024-longrag}, and \citet{jin2025longcontext}—have proposed methods to improve the effectiveness of LLMs in long-context settings. In parallel, \citet{lee2024longcontextlanguagemodelssubsume} introduced LOFT, a new benchmark designed to evaluate LLMs on a broad range of tasks addressable by either RAG or long-context modeling.

\paragraph{Summarization} Summarization has been a long-standing challenge in natural language processing. Early benchmark datasets, such as CNN/Daily Mail \cite{see-etal-2017-get} and XSum \cite{Narayan2018DontGM}, primarily targeted single-document summarization. Subsequent efforts, including MultiNews \cite{fabbri-etal-2019-multi} and MS$^2$ \cite{deyoung-etal-2021-ms}, extended this task to the multi-document setting. Another line of related work focuses on query-based summarization, for which QMSum \cite{zhong-etal-2021-qmsum} and DUC 2005 \cite{10.5555/1654679.1654689} are two widely used datasets.

\paragraph{Text to SQL} Text-to-SQL is a widely studied approach for tackling aggregative question answering. In this paradigm, the model is required to generate a structured database query based on a natural language question. Several established benchmarks have been proposed to evaluate this task, including WikiSQL \cite{zhongSeq2SQL2017}, Spider \cite{lei2024spider}, BIRD \cite{li2024can}, and WikiTableQA \cite{pasupat-liang-2015-compositional}. Additionally, LOFT \cite{lee2024longcontextlanguagemodelssubsume} includes a sub-task specifically designed to assess how effectively large language models can emulate database-style querying.
