# Supplementary material for: Interactive Training: Feedback-Driven Neural Network Optimization
Source: arXiv:2510.02297 source file (2025-10-02)
Supplement: Supplementary file 5 [file question_table.tex]

\begin{table}[ht]
\centering
\begin{tabularx}{\columnwidth}{>{\raggedright\arraybackslash}X l r}
\toprule
Condition & Target & Count \\
\midrule
 \multicolumn{3}{c}{0 Condition}   \\
\midrule
none & topic & 1 \\ 
none & loc & 1 \\ 
none & lang & 1 \\ 
\midrule
 \multicolumn{3}{c}{1 Condition}   \\
\midrule
user & keywords & 370 \\ 
user & time & 100 \\ 
keywords & user & 96 \\ 
user & lang & 60 \\ 
user & topic & 54 \\ 
time & user & 39 \\ 
topic & subtopic & 26 \\ 
loc & topic & 20 \\ 
loc & keywords & 17 \\ 
lang & topic & 9 \\ 
time & topic & 6 \\ 
time & keywords & 6 \\ 
topic & loc & 6 \\ 
topic & user & 6 \\ 
topic & lang & 4 \\ 
topic & keywords & 4 \\ 
time & lang & 4 \\ 
lang & keywords & 1 \\ 
\midrule
 \multicolumn{3}{c}{2 Conditions}   \\
\midrule
user, topic & subtopic & 199 \\ 
user, topic & keywords & 185 \\ 
user, user & subtopic & 141 \\ 
user, topic & time & 114 \\ 
topic, lang & subtopic & 100 \\ 
time, topic & user & 98 \\ 
time, topic & subtopic & 98 \\ 
topic, lang & user & 98 \\ 
topic, loc & time & 97 \\ 
topic, keywords & user & 97 \\ 
\bottomrule
\end{tabularx}
\caption{Question Type Statistics}
\label{tab:data_question_stat}
\end{table}

\begin{table}[!t]
\centering
\begin{tabularx}{\columnwidth}{>{\raggedright\arraybackslash}X l r}
\toprule
Condition & Target & Count \\
\midrule
topic, loc & subtopic & 96 \\ 
topic, keywords & time & 96 \\ 
time, user & keywords & 94 \\ 
topic, subtopic & user & 93 \\ 
subtopic, subtopic & user & 93 \\ 
topic, loc & keywords & 82 \\ 
topic, lang & time & 74 \\ 
time, topic & loc & 60 \\
topic, subtopic & keywords & 55 \\ 
topic, topic & user & 55 \\ 
time, user & topic & 53 \\ 
user, user & topic & 53 \\ 
time, topic & keywords & 49 \\ 
topic, subtopic & loc & 39 \\ 
time, loc & topic & 34 \\ 
time, lang & topic & 31 \\ 
topic, lang & keywords & 27 \\ 
time, topic & lang & 15 \\ 
topic, subtopic & lang & 13 \\ 
topic, loc & user & 10 \\ 
\midrule
 \multicolumn{3}{c}{3 Conditions}   \\
\midrule
loc, topic, subtopic & user & 287 \\ 
lang, topic, subtopic & user & 284 \\ 
user, topic, subtopic & keywords & 276 \\ 
time, loc, topic & user & 199 \\ 
time, topic, subtopic & keywords & 175 \\ 
user, user, user & subtopic & 132 \\ 
user, topic, keywords & time & 114 \\ 
time, topic, keywords & user & 100 \\ 
time, loc, topic & subtopic & 100 \\ 
time, user, topic & subtopic & 100 \\ 
loc, topic, keywords & user & 99 \\ 
user, topic, subtopic & time & 98 \\ 
user, topic, keywords & subtopic & 98 \\ 
loc, topic, keywords & time & 98 \\ 
lang, topic, keywords & time & 98 \\ 
time, topic, subtopic & user & 97 \\ 
lang, topic, keywords & user & 96 \\ 
topic, subtopic, keywords & user & 94 \\ 
loc, topic, subtopic & keywords & 93 \\ 
lang, topic, subtopic & keywords & 82 \\ 
time, topic, subtopic & loc & 76 \\ 
user, user, user & topic & 51 \\ 

\bottomrule
\end{tabularx}
\end{table}
